# Supplementary material for: Uniform electron gases: III. Low-density gases on three-dimensional spheres
Source: arXiv:1508.02491 source file (2015-08-12)
Supplement: Supplementary file 1 [file Supplementary_Materials.pdf]

# Supplementary Material for "Correlation energies of low-density electron gases on three-dimensional spheres"

Davids Agboola,[1] Anneke Knol,[1] Peter M.W. Gill,[1, a)] and Pierre-François Loos[1, b)]

*Research School of Chemistry, Australian National University, ACT 2601, Australia*

---

[a)] Electronic mail: peter.gill@anu.edu.au

[b)] Corresponding author; Electronic mail: pf.loos@anu.edu.au

TABLE I: Cartesian coordinates of uniform Thomson lattices on a 3-sphere. For brevity, the points $(-w, -x, -y, -z)$ are not listed for $n = 24$ and 48. For $n = 12$, $c = \cos\theta$, $s = \sin\theta$ and $\theta = 0.7935536685\ldots$ For $n = 48$, $s_k = \sin(k\pi/12)/\sqrt{2}$.

| | $w$ | $x$ | $y$ | $z$ |
|---|---|---|---|---|
| $n = 2$ | 0 | 0 | 0 | $+1$ |
| | 0 | 0 | 0 | $-1$ |
| $n = 3$ | 0 | 0 | 0 | $+1$ |
| | 0 | 0 | $+\sqrt{3}/2$ | $-1/2$ |
| | 0 | 0 | $-\sqrt{3}/2$ | $-1/2$ |
| $n = 4$ | 0 | $+1/\sqrt{3}$ | $+1/\sqrt{3}$ | $+1/\sqrt{3}$ |
| | 0 | $+1/\sqrt{3}$ | $-1/\sqrt{3}$ | $-1/\sqrt{3}$ |
| | 0 | $-1/\sqrt{3}$ | $+1/\sqrt{3}$ | $-1/\sqrt{3}$ |
| | 0 | $-1/\sqrt{3}$ | $-1/\sqrt{3}$ | $+1/\sqrt{3}$ |
| $n = 5$ | 0 | 0 | 0 | $+1$ |
| | $+\sqrt{5}/4$ | $+\sqrt{5}/4$ | $+\sqrt{5}/4$ | $-1/4$ |
| | $+\sqrt{5}/4$ | $-\sqrt{5}/4$ | $-\sqrt{5}/4$ | $-1/4$ |
| | $-\sqrt{5}/4$ | $+\sqrt{5}/4$ | $-\sqrt{5}/4$ | $-1/4$ |
| | $-\sqrt{5}/4$ | $-\sqrt{5}/4$ | $+\sqrt{5}/4$ | $-1/4$ |
| $n = 6$ | 0 | 0 | 0 | $+1$ |
| | 0 | 0 | $+\sqrt{3}/2$ | $-1/2$ |
| | 0 | 0 | $-\sqrt{3}/2$ | $-1/2$ |
| | 0 | $+1$ | 0 | 0 |
| | $+\sqrt{3}/2$ | $-1/2$ | 0 | 0 |
| | $-\sqrt{3}/2$ | $-1/2$ | 0 | 0 |
| $n = 8$ | 0 | 0 | 0 | $\pm 1$ |
| | 0 | 0 | $\pm 1$ | 0 |
| | 0 | $\pm 1$ | 0 | 0 |
| | $\pm 1$ | 0 | 0 | 0 |
| $n = 10$ | 0 | 0 | 0 | $+1$ |

TABLE I: (continued)

| | $w$ | $x$ | $y$ | $z$ |
|---|---|---|---|---|
| | $0$ | $0$ | $\sin(2\pi/5)$ | $\cos(2\pi/5)$ |
| | $0$ | $0$ | $\sin(4\pi/5)$ | $\cos(4\pi/5)$ |
| | $0$ | $0$ | $\sin(6\pi/5)$ | $\cos(6\pi/5)$ |
| | $0$ | $0$ | $\sin(8\pi/5)$ | $\cos(8\pi/5)$ |
| | $0$ | $-1$ | $0$ | $0$ |
| | $\sin(2\pi/5)$ | $-\cos(2\pi/5)$ | $0$ | $0$ |
| | $\sin(4\pi/5)$ | $-\cos(4\pi/5)$ | $0$ | $0$ |
| | $\sin(6\pi/5)$ | $-\cos(6\pi/5)$ | $0$ | $0$ |
| | $\sin(8\pi/5)$ | $-\cos(8\pi/5)$ | $0$ | $0$ |
| $n = 12$ | $+c$ | $0$ | $+s$ | $0$ |
| | $+c$ | $0$ | $-s/2$ | $+\sqrt{3}s/2$ |
| | $+c$ | $0$ | $-s/2$ | $-\sqrt{3}s/2$ |
| | $-c$ | $0$ | $+s$ | $0$ |
| | $-c$ | $0$ | $-s/2$ | $+\sqrt{3}s/2$ |
| | $-c$ | $0$ | $-s/2$ | $-\sqrt{3}s/2$ |
| | $0$ | $+c$ | $-s$ | $0$ |
| | $0$ | $+c$ | $+s/2$ | $+\sqrt{3}s/2$ |
| | $0$ | $+c$ | $+s/2$ | $-\sqrt{3}s/2$ |
| | $0$ | $-c$ | $-s$ | $0$ |
| | $0$ | $-c$ | $+s/2$ | $+\sqrt{3}s/2$ |
| | $0$ | $-c$ | $+s/2$ | $-\sqrt{3}s/2$ |

TABLE I: (continued)

| | $w$ | $x$ | $y$ | $z$ |
|---|---|---|---|---|
| $n = 13$ | 1 | 0 | 0 | 0 |
| | 0.344301 | 0.223764 | 0.911804 | 0 |
| | 0.344301 | 0.223764 | −0.911804 | 0 |
| | 0.344301 | −0.223764 | 0 | 0.911804 |
| | 0.344301 | −0.223764 | 0 | −0.911804 |
| | 0.0684726 | 0.816983 | −0.151254 | 0.552243 |
| | 0.0684726 | 0.816983 | 0.151254 | −0.552243 |
| | 0.0684726 | −0.816983 | 0.552243 | 0.151254 |
| | 0.0684726 | −0.816983 | −0.552243 | −0.151254 |
| | −0.662773 | 0.308168 | 0.552243 | 0.400989 |
| | −0.662773 | 0.308168 | −0.552243 | −0.400989 |
| | −0.662773 | −0.308168 | −0.400989 | 0.552243 |
| | −0.662773 | −0.308168 | 0.400989 | −0.552243 |
| $n = 24$ | 0 | 0 | 0 | +1 |
| | 0 | 0 | +1 | 0 |
| | 0 | +1 | 0 | 0 |
| | +1 | 0 | 0 | 0 |
| | +1/2 | +1/2 | +1/2 | +1/2 |
| | +1/2 | +1/2 | +1/2 | −1/2 |
| | +1/2 | +1/2 | −1/2 | +1/2 |
| | +1/2 | +1/2 | −1/2 | −1/2 |
| | +1/2 | −1/2 | +1/2 | +1/2 |
| | +1/2 | −1/2 | +1/2 | −1/2 |
| | +1/2 | −1/2 | −1/2 | +1/2 |
| | +1/2 | −1/2 | −1/2 | −1/2 |
| $n = 48$ | 0 | 0 | 0 | +1 |
| | 0 | 0 | +1 | 0 |
| | 0 | +1 | 0 | 0 |

TABLE I: (continued)

| $w$ | $x$ | $y$ | $z$ |
|---|---|---|---|
| $+1$ | $0$ | $0$ | $0$ |
| $0$ | $0$ | $+1/\sqrt{2}$ | $+1/\sqrt{2}$ |
| $0$ | $0$ | $+1/\sqrt{2}$ | $-1/\sqrt{2}$ |
| $+1/\sqrt{2}$ | $+1/\sqrt{2}$ | $0$ | $0$ |
| $+1/\sqrt{2}$ | $-1/\sqrt{2}$ | $0$ | $0$ |
| $-s_1$ | $+s_5$ | $+s_4$ | $+s_2$ |
| $+s_1$ | $-s_5$ | $+s_4$ | $+s_2$ |
| $+s_1$ | $+s_5$ | $-s_4$ | $+s_2$ |
| $+s_1$ | $+s_5$ | $+s_4$ | $-s_2$ |
| $-s_5$ | $+s_1$ | $+s_2$ | $+s_4$ |
| $+s_5$ | $-s_1$ | $+s_2$ | $+s_4$ |
| $+s_5$ | $+s_1$ | $-s_2$ | $+s_4$ |
| $+s_5$ | $+s_1$ | $+s_2$ | $-s_4$ |
| $+s_2$ | $+s_4$ | $+s_1$ | $+s_5$ |
| $+s_2$ | $+s_4$ | $-s_1$ | $-s_5$ |
| $+s_2$ | $-s_4$ | $+s_1$ | $-s_5$ |
| $+s_2$ | $-s_4$ | $-s_1$ | $+s_5$ |
| $+s_4$ | $+s_2$ | $+s_5$ | $+s_1$ |
| $+s_4$ | $+s_2$ | $-s_5$ | $-s_1$ |
| $+s_4$ | $-s_2$ | $+s_5$ | $-s_1$ |
| $+s_4$ | $-s_2$ | $-s_5$ | $+s_1$ |
